# Supplementary material for: Feasibility Study of Measuring $\Lambda^0\to n\pi^{0}$ Using a High-Granularity Zero-Degree Calorimeter at the Future Electron-Ion Collider
Source: arXiv:2412.12346 source file (2025-03-11)
Supplement: Supplementary file 1 [file appendix.tex]

% \appendix
% \section{Combinatoric noise}
% In this appendix we estimate how well combinatorical background can be removed.  We generated a sample of 10k fake events with neutrons and 2 photons.  The energies  with energies log-uniform distributed from 100 to 250 GeV and 5 to 60 GeV for the neutrons and protons, respectively, with their positions uniformly distributed within the fiducial disk of the ZDC.  

% We then ran the IDOLA algorithm on this fake sample, using 10 iterations.  The distributions of the $\pi^0$ mass, the $\Lambda^0$ mass, and the vertex positions of these events are shown in Fig.~\ref{fig:combinatoric}.

% We note that the $\pi^0$ mass does not converge as well in these events as in the $\Lambda^0\rightarrow n\gamma\gamma$ events.  In the $\Lambda^0\rightarrow n\gamma\gamma$ events, the $\pi^0$ mass distribution, after 10 iterations, has a nearly Gaussian shape, with $\sigma\approx 0.4$ MeV, whereas in the combinatoric events, the mass is much more spread out.  Further, in the reconstructed $\Lambda^0$ mass distribution, the combinatoric events have a wide tail to the right, indicating that the mass is more likely to be reconstructed as larger than in real life than in 
